# Supplementary material for: Chordless cycle filtrations for dimensionality detection in complex networks via topological data analysis
Source: arXiv:2509.08350 source file (2026-05-08)
Supplement: Supplementary file 1 [file SI_TDA.pdf]

# Supplementary Information for “Chordless cycle filtrations for dimensionality detection in complex networks via topological data analysis”

Aina Ferrà Marcús,<sup>1</sup> Robert Jankowski,<sup>2,3</sup> Meritxell Vila Miñana,<sup>4</sup> Carles Casacuberta,<sup>1</sup> and M. Ángeles Serrano<sup>2,3,5</sup>

<sup>1</sup>*Departament de Matemàtiques i Informàtica, Universitat de Barcelona,  
Gran Via de les Corts Catalanes 585, 08007 Barcelona, Spain*

<sup>2</sup>*Departament de Física de la Matèria Condensada,  
Universitat de Barcelona, Martí i Franquès 1, E-08028 Barcelona, Spain*

<sup>3</sup>*Universitat de Barcelona Institute of Complex Systems (UBICS), Universitat de Barcelona, Barcelona, Spain*

<sup>4</sup>*Center for Complex Networks and Systems Research, Luddy School of Informatics,  
Computing, and Engineering, Indiana University, Bloomington, IN, USA*

<sup>5</sup>*ICREA, Passeig Lluís Companys 23, E-08010 Barcelona, Spain\**

## CONTENTS

|                                                                            |    |
|----------------------------------------------------------------------------|----|
| 1. Dimensionality estimation of real networks with persistence descriptors | 2  |
| 2. Neural network architecture and predictions                             | 4  |
| 3. Topological properties of real networks and their inferred dimensions   | 7  |
| 4. Network generation algorithms                                           | 11 |
| Supplementary References                                                   | 11 |

---

\* marian.serrano@ub.edu

## 1. DIMENSIONALITY ESTIMATION OF REAL NETWORKS WITH PERSISTENCE DESCRIPTORS

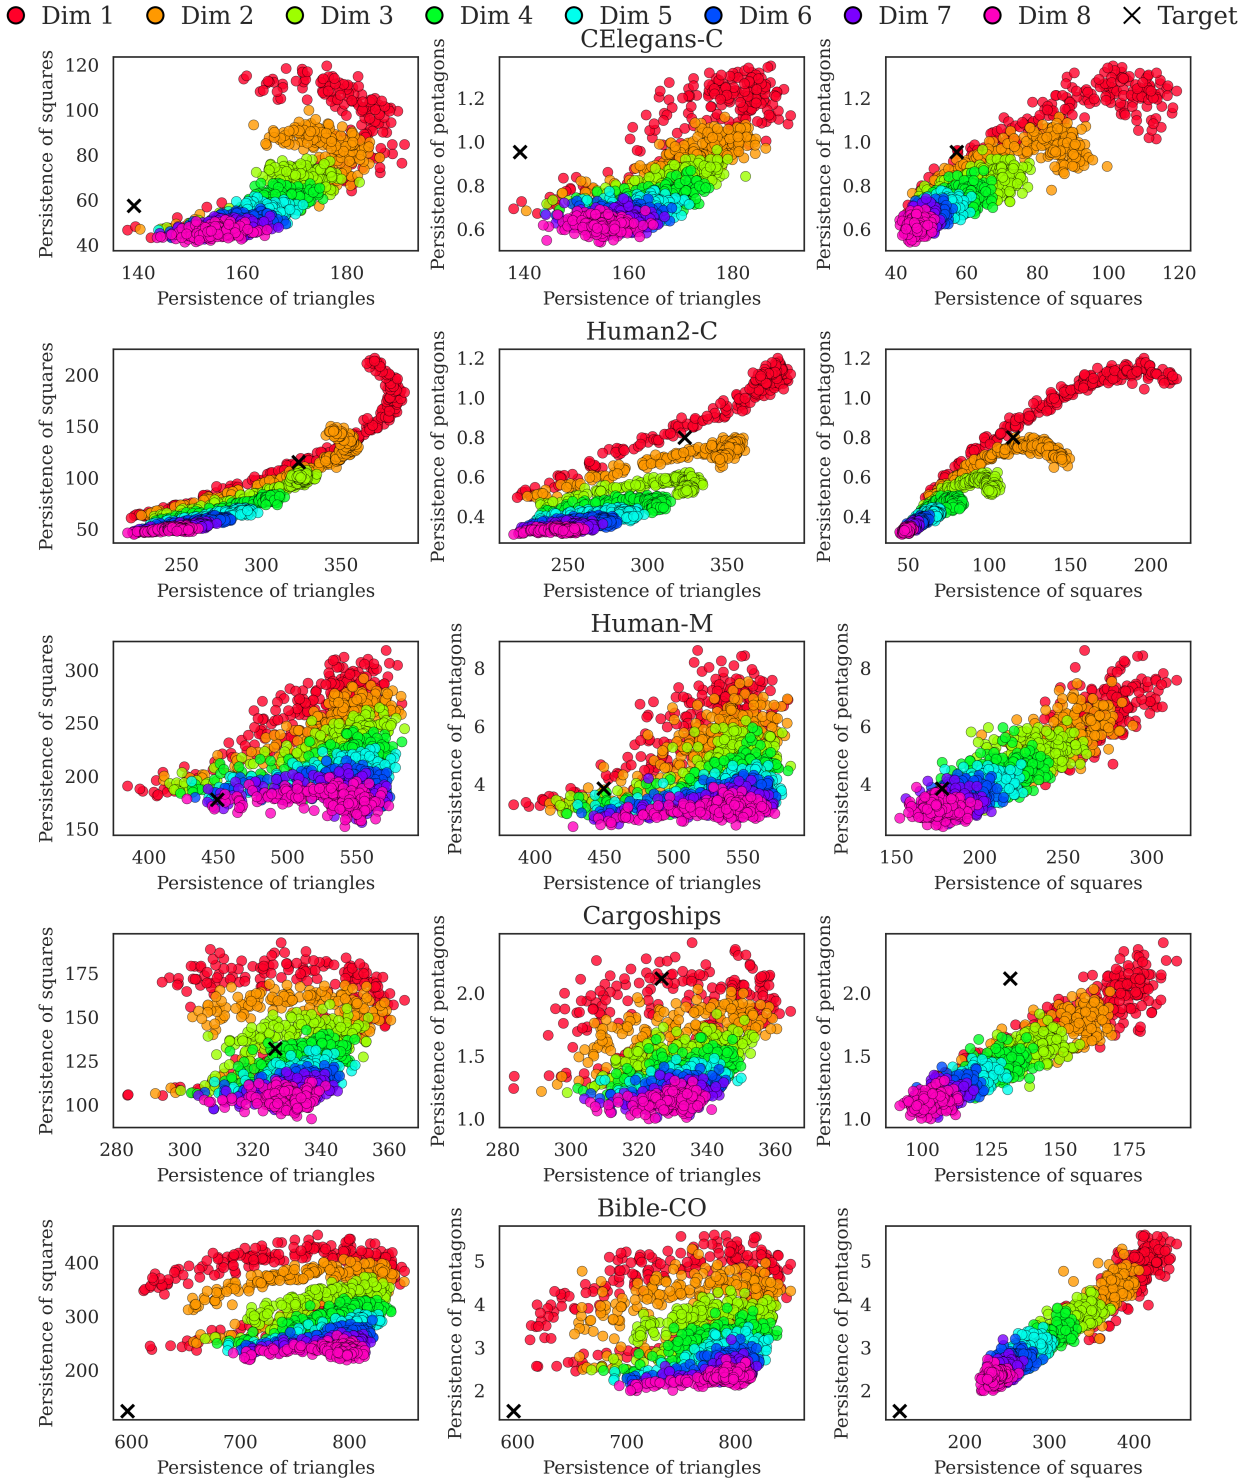

FIG. S1: 2D projections representing an ensemble of 1330 surrogates for each real network in the phase space of total persistence computed from three chordless cycle densities (triangles, squares, and pentagons). Points are colored by dimension, and the target network is marked with a black cross. Part 1 of 2.

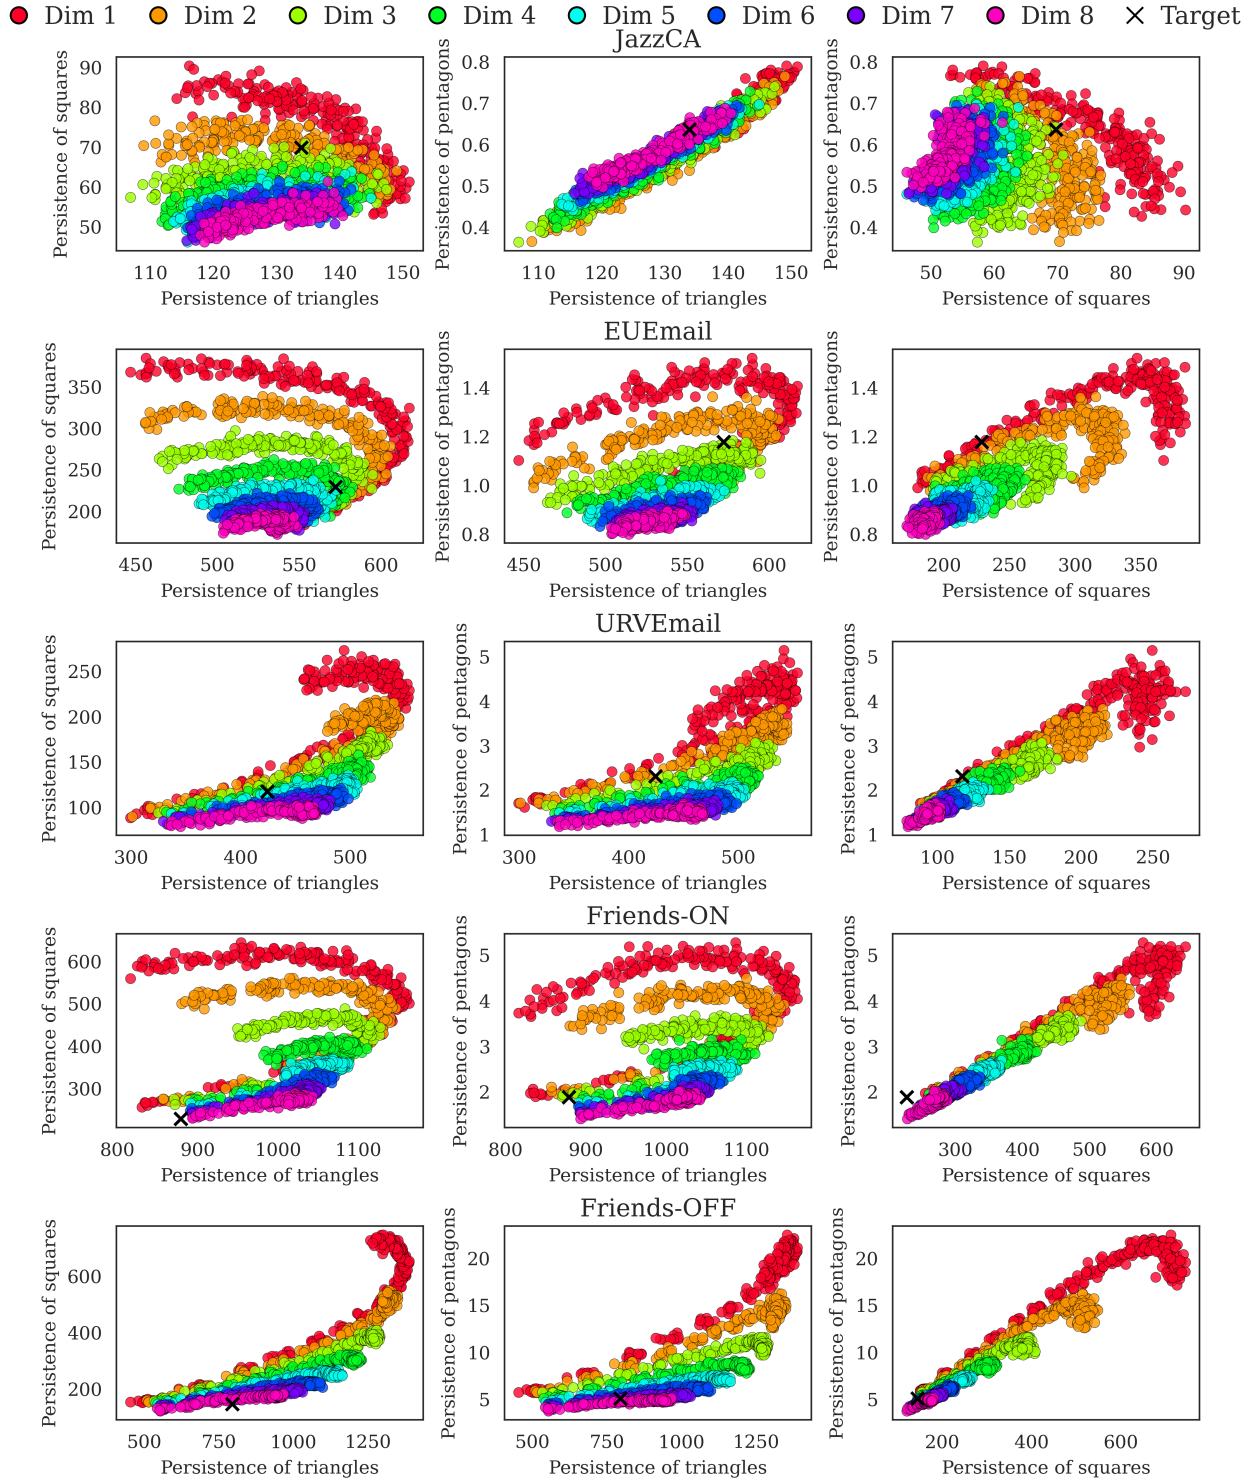

FIG. S2: 2D projections representing an ensemble of 1330 surrogates for each real network in the phase space of total persistence computed from three chordless cycle densities (triangles, squares, and pentagons). Points are colored by dimension, and the target network is marked with a black cross. Part 2 of 2.

## 2. NEURAL NETWORK ARCHITECTURE AND PREDICTIONS

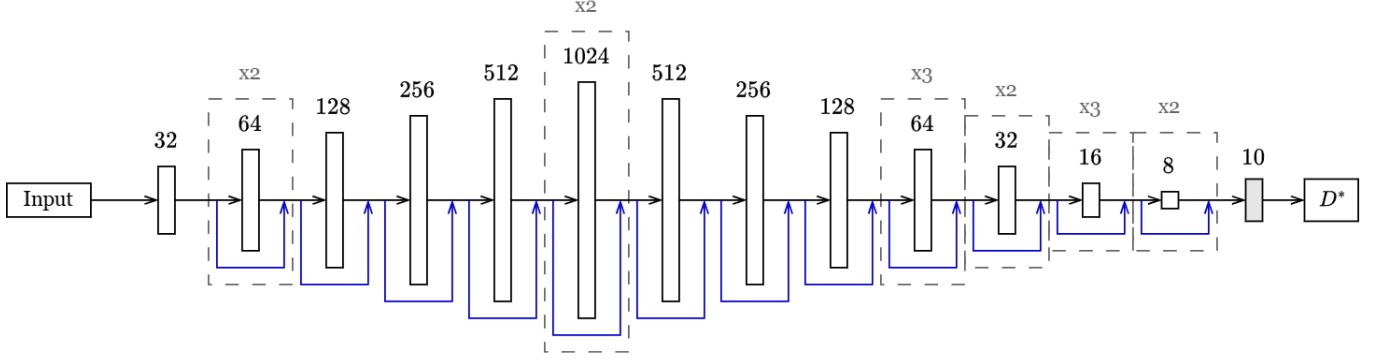

FIG. S3: Schematic representation of the DIMNN neural network architecture. Boxes indicate layers within the MLP, with the number above each box specifying the number of neurons in that layer. Blue arrows are used to denote skip (residual) connections. Dashed gray boxes denote repeated layer blocks, with the repetition count indicated above each block. The output layer is shaded in gray and employs a softmax activation, yielding a 10-dimensional output corresponding to the number of classes in the classification problem.

TABLE S1: Validation accuracies after five repetitions of DIMNN, a ResNet training with AdamW optimizer using the SYNNET network database. Columns correspond to features included in each model:  $N$  number of nodes,  $\langle k \rangle$  average degree,  $\langle k^2 \rangle / \langle k \rangle^2$  normalized second moment,  $k_{\min}$  minimum degree,  $k_{\max}$  maximum degree,  $\langle k_{\text{nn}} \rangle$  mean average neighbor degree,  $C_t$  average triangle density,  $C_s$  average chordless square density,  $C_p$  average chordless pentagon density,  $TP_t$ ,  $TP_s$ ,  $TP_p$  total persistence in homological dimension 1 computed from chordless cycle filtrations (triangles, squares, and pentagons, respectively).

| $N$ | $\langle k \rangle$ | $\langle k^2 \rangle / \langle k \rangle^2$ | $k_{\min}$ | $k_{\max}$ | $\langle k_{\text{nn}} \rangle$ | $C_t$ | $C_s$ | $C_p$ | $TP_t$ | $TP_s$ | $TP_p$ | Accuracy (%)                       | Time (sec) | Epochs |
|-----|---------------------|---------------------------------------------|------------|------------|---------------------------------|-------|-------|-------|--------|--------|--------|------------------------------------|------------|--------|
|     |                     |                                             |            |            |                                 | ✓     | ✓     | ✓     |        |        |        | $53.20 \pm 2.15$                   | 7529.71    | 73.40  |
| ✓   |                     |                                             |            |            |                                 | ✓     | ✓     | ✓     |        |        |        | $66.79 \pm 0.67$                   | 7582.86    | 73.60  |
| ✓   | ✓                   |                                             |            |            |                                 | ✓     | ✓     | ✓     |        |        |        | $68.95 \pm 2.08$                   | 5718.05    | 55.50  |
| ✓   | ✓                   | ✓                                           |            |            |                                 | ✓     | ✓     | ✓     |        |        |        | $81.53 \pm 0.67$                   | 6372.85    | 61.40  |
| ✓   | ✓                   | ✓                                           | ✓          | ✓          |                                 | ✓     | ✓     | ✓     |        |        |        | $80.96 \pm 0.46$                   | 5449.96    | 52.75  |
| ✓   | ✓                   | ✓                                           | ✓          | ✓          | ✓                               | ✓     | ✓     | ✓     |        |        |        | $82.32 \pm 1.39$                   | 4890.98    | 47.40  |
|     |                     |                                             |            |            |                                 |       |       |       | ✓      | ✓      | ✓      | $56.06 \pm 1.17$                   | 8326.58    | 74.40  |
| ✓   |                     |                                             |            |            |                                 |       |       |       | ✓      | ✓      | ✓      | $59.02 \pm 2.73$                   | 6348.86    | 65.00  |
| ✓   | ✓                   |                                             |            |            |                                 |       |       |       | ✓      | ✓      | ✓      | $59.45 \pm 1.52$                   | 6015.84    | 60.00  |
| ✓   | ✓                   | ✓                                           |            |            |                                 |       |       |       | ✓      | ✓      | ✓      | $71.60 \pm 2.30$                   | 6563.73    | 64.67  |
| ✓   | ✓                   | ✓                                           | ✓          | ✓          |                                 |       |       |       | ✓      | ✓      | ✓      | $70.74 \pm 2.57$                   | 6663.77    | 65.80  |
| ✓   | ✓                   | ✓                                           | ✓          | ✓          | ✓                               |       |       |       | ✓      | ✓      | ✓      | $73.10 \pm 1.19$                   | 5592.25    | 54.80  |
|     |                     |                                             |            |            |                                 | ✓     | ✓     | ✓     | ✓      | ✓      | ✓      | $72.64 \pm 3.32$                   | 6518.76    | 59.20  |
| ✓   |                     |                                             |            |            |                                 | ✓     | ✓     | ✓     | ✓      | ✓      | ✓      | $74.57 \pm 1.86$                   | 6343.14    | 57.00  |
| ✓   | ✓                   |                                             |            |            |                                 | ✓     | ✓     | ✓     | ✓      | ✓      | ✓      | $74.39 \pm 2.76$                   | 7928.53    | 59.40  |
| ✓   | ✓                   | ✓                                           |            |            |                                 | ✓     | ✓     | ✓     | ✓      | ✓      | ✓      | $81.83 \pm 0.44$                   | 7682.31    | 53.00  |
| ✓   | ✓                   | ✓                                           | ✓          | ✓          |                                 | ✓     | ✓     | ✓     | ✓      | ✓      | ✓      | $81.41 \pm 0.38$                   | 5778.89    | 37.60  |
| ✓   | ✓                   | ✓                                           | ✓          | ✓          | ✓                               | ✓     | ✓     | ✓     | ✓      | ✓      | ✓      | <b><math>83.00 \pm 0.38</math></b> | 4796.51    | 42.60  |



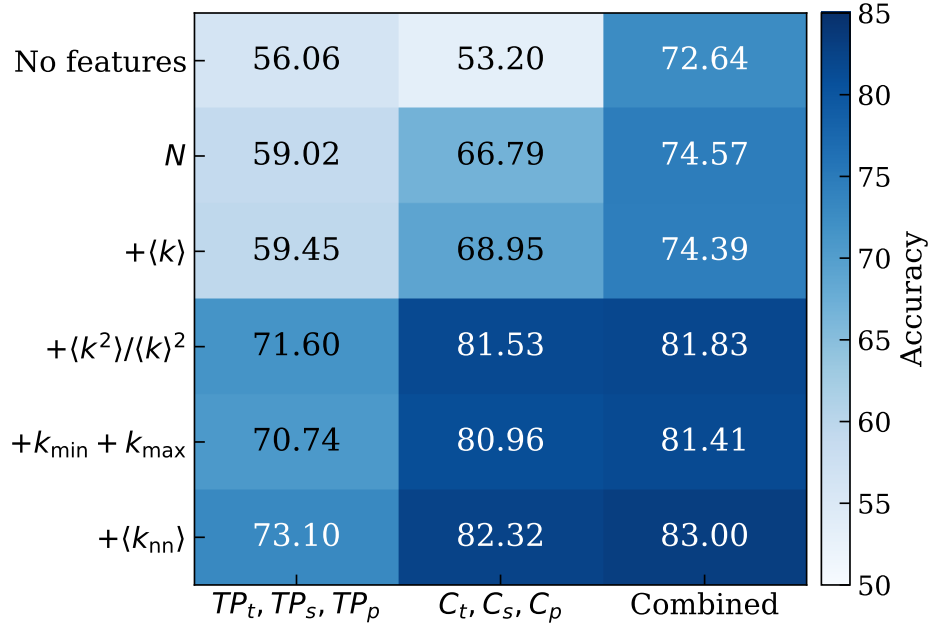

FIG. S4: Impact of cycle density and TDA features on DIMNN validation accuracy on the SYNNET dataset. Heatmap of mean validation accuracy for five progressively enriched input network features. The results are averaged over five neural network initializations.

TABLE S2: Comparative measures for each combination of graph features between the predictions of the DIMNN classifier and a regressor with the same architecture and mean squared error as loss function, averaged over five repetitions. Discrepancy is computed from the collection of SYNNET networks in the validation set on which the two models do not agree. *Agreement (%)*: Percentage of agreement between the two models; *Median*: Median discrepancy; *Q3*: Third quartile of discrepancy; *Mean*: Mean of discrepancy; *Std*: Standard deviation of discrepancy.

| Descriptors                                                                                                                                    | Agreement (%) | Median | Q3  | Mean | Std  |
|------------------------------------------------------------------------------------------------------------------------------------------------|---------------|--------|-----|------|------|
| $C_t, C_s, C_p$                                                                                                                                | 44.31         | 1.0    | 2.0 | 1.41 | 0.69 |
| $N, C_t, C_s, C_p$                                                                                                                             | 67.12         | 1.0    | 1.0 | 1.19 | 0.46 |
| $N, \langle k \rangle, C_t, C_s, C_p$                                                                                                          | 73.18         | 1.0    | 1.0 | 1.18 | 0.45 |
| $N, \langle k \rangle, \langle k^2 \rangle / \langle k \rangle^2, C_t, C_s, C_p$                                                               | 88.45         | 1.0    | 1.0 | 1.04 | 0.24 |
| $N, \langle k \rangle, \langle k^2 \rangle / \langle k \rangle^2, k_{\min}, k_{\max}, C_t, C_s, C_p$                                           | 88.19         | 1.0    | 1.0 | 1.06 | 0.30 |
| $N, \langle k \rangle, \langle k^2 \rangle / \langle k \rangle^2, k_{\min}, k_{\max}, \langle k_{nn} \rangle, C_t, C_s, C_p$                   | 88.90         | 1.0    | 1.0 | 1.05 | 0.27 |
| $TP_t, TP_s, TP_p$                                                                                                                             | 58.83         | 1.0    | 1.4 | 1.30 | 0.63 |
| $N, TP_t, TP_s, TP_p$                                                                                                                          | 67.75         | 1.0    | 1.0 | 1.22 | 0.56 |
| $N, \langle k \rangle, TP_t, TP_s, TP_p$                                                                                                       | 71.06         | 1.0    | 1.0 | 1.18 | 0.48 |
| $N, \langle k \rangle, \langle k^2 \rangle / \langle k \rangle^2, TP_t, TP_s, TP_p$                                                            | 79.14         | 1.0    | 1.0 | 1.12 | 0.39 |
| $N, \langle k \rangle, \langle k^2 \rangle / \langle k \rangle^2, k_{\min}, k_{\max}, TP_t, TP_s, TP_p$                                        | 77.70         | 1.0    | 1.0 | 1.12 | 0.40 |
| $N, \langle k \rangle, \langle k^2 \rangle / \langle k \rangle^2, k_{\min}, k_{\max}, \langle k_{nn} \rangle, TP_t, TP_s, TP_p$                | 80.43         | 1.0    | 1.0 | 1.11 | 0.40 |
| $C_t, C_s, C_p, TP_t, TP_s, TP_p$                                                                                                              | 79.33         | 1.0    | 1.0 | 1.05 | 0.24 |
| $N, C_t, C_s, C_p, TP_t, TP_s, TP_p$                                                                                                           | 79.62         | 1.0    | 1.0 | 1.06 | 0.27 |
| $N, \langle k \rangle, C_t, C_s, C_p, TP_t, TP_s, TP_p$                                                                                        | 78.65         | 1.0    | 1.0 | 1.05 | 0.24 |
| $N, \langle k \rangle, \langle k^2 \rangle / \langle k \rangle^2, C_t, C_s, C_p, TP_t, TP_s, TP_p$                                             | 88.38         | 1.0    | 1.0 | 1.04 | 0.24 |
| $N, \langle k \rangle, \langle k^2 \rangle / \langle k \rangle^2, k_{\min}, k_{\max}, C_t, C_s, C_p, TP_t, TP_s, TP_p$                         | 87.79         | 1.0    | 1.0 | 1.06 | 0.28 |
| $N, \langle k \rangle, \langle k^2 \rangle / \langle k \rangle^2, k_{\min}, k_{\max}, \langle k_{nn} \rangle, C_t, C_s, C_p, TP_t, TP_s, TP_p$ | 88.86         | 1.0    | 1.0 | 1.05 | 0.25 |

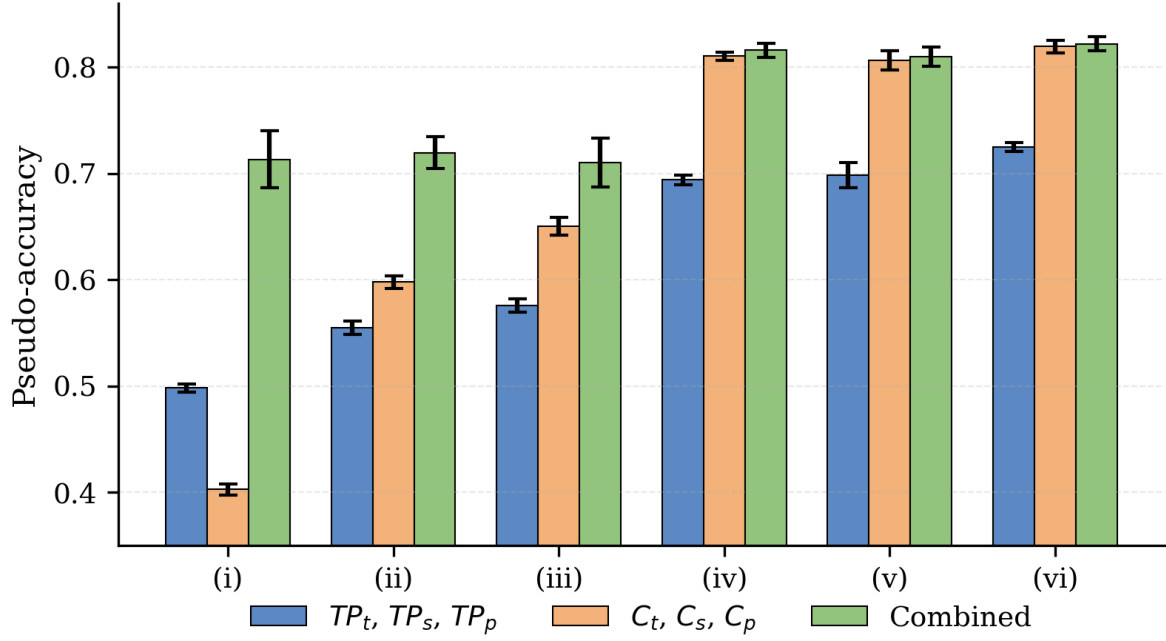

FIG. S5: Averages and standard deviations of pseudo-accuracy on a validation set after five runs of a neural network regressor using the SYNNET database. Pseudo-accuracy refers to the fact that the prediction of a regressor is a real number, which is approximated to the nearest integer. *Blue*: Accuracies obtained using total persistences  $TP_t$ ,  $TP_s$ ,  $TP_p$ , plus cumulative features. *Orange*: Accuracies using average cycle densities  $C_t$ ,  $C_s$ ,  $C_p$ , plus cumulative features. *Green*: Accuracies obtained by combining total persistences and mean cycle densities plus cumulative features. Successive columns correspond to incorporating one after the other the following additional features into the model: (i) no added features; (ii) number of nodes  $N$ ; (iii) number of nodes and average degree  $\langle k \rangle$ ; (iv) number of nodes, average degree, and normalized second moment  $\langle k^2 \rangle / \langle k \rangle^2$ ; (v) number of nodes, average degree, normalized second moment, minimum degree  $k_{\min}$  and maximum degree  $k_{\max}$ ; (vi) number of nodes, average degree, normalized second moment, minimum degree, maximum degree, and mean average neighbor degree  $\langle k_{nn} \rangle$ .

### 3. TOPOLOGICAL PROPERTIES OF REAL NETWORKS AND THEIR INFERRED DIMENSIONS

We compile a dataset of 53 real-world networks from various domains. For more details about each network, we refer to [1] and [2].

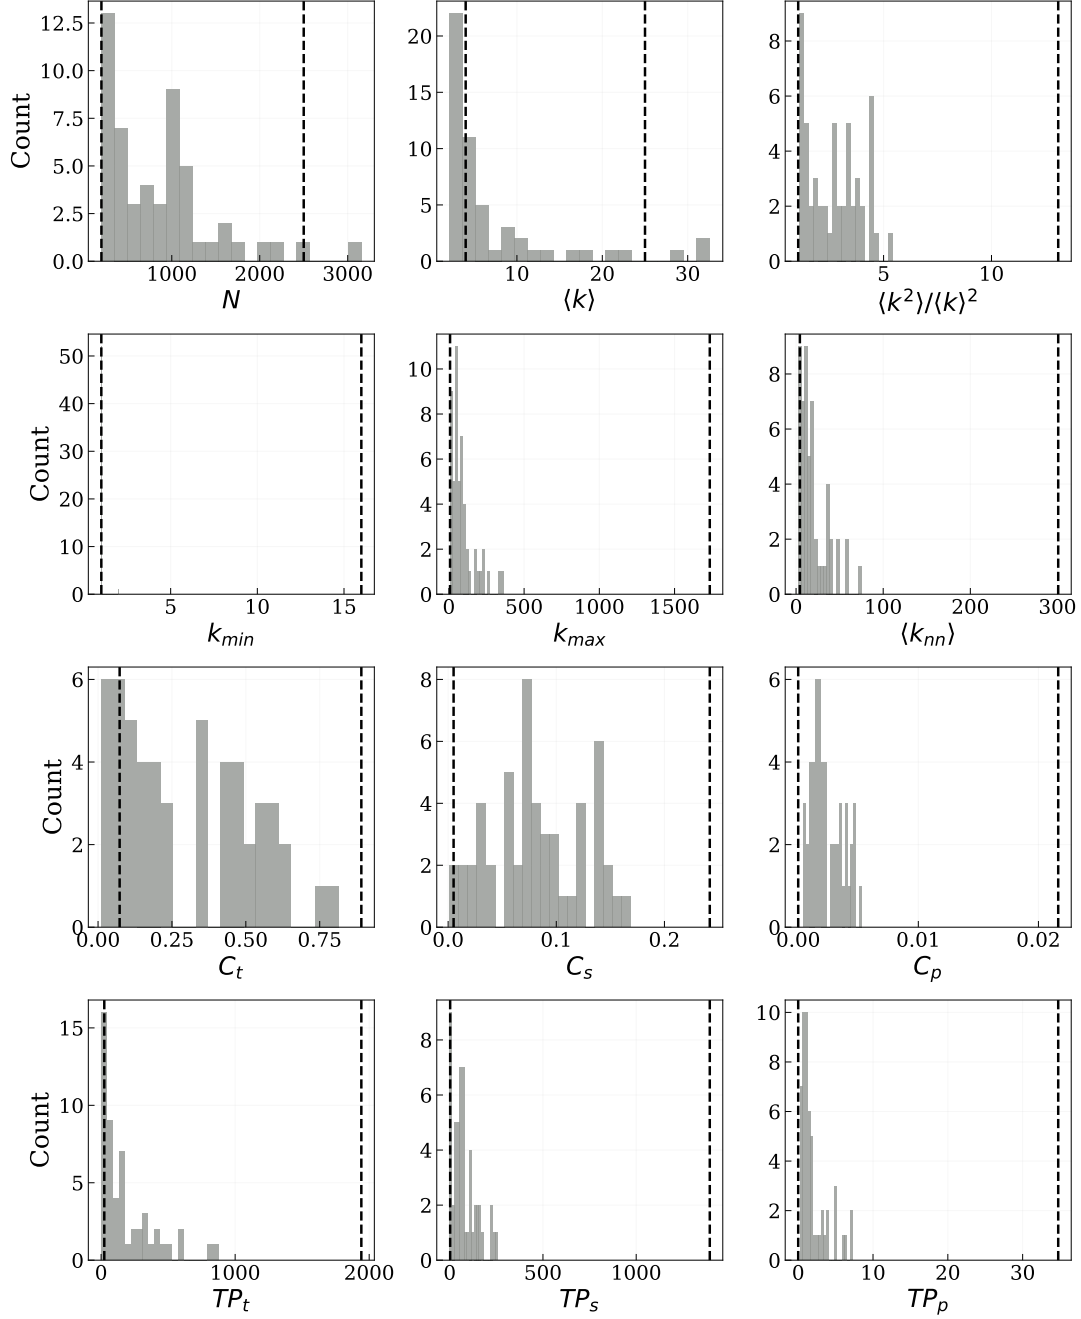

FIG. S6: Distributions of the topological properties of real networks. The dotted black lines in each panel indicate the minimum and maximum value of a given feature in the training dataset.

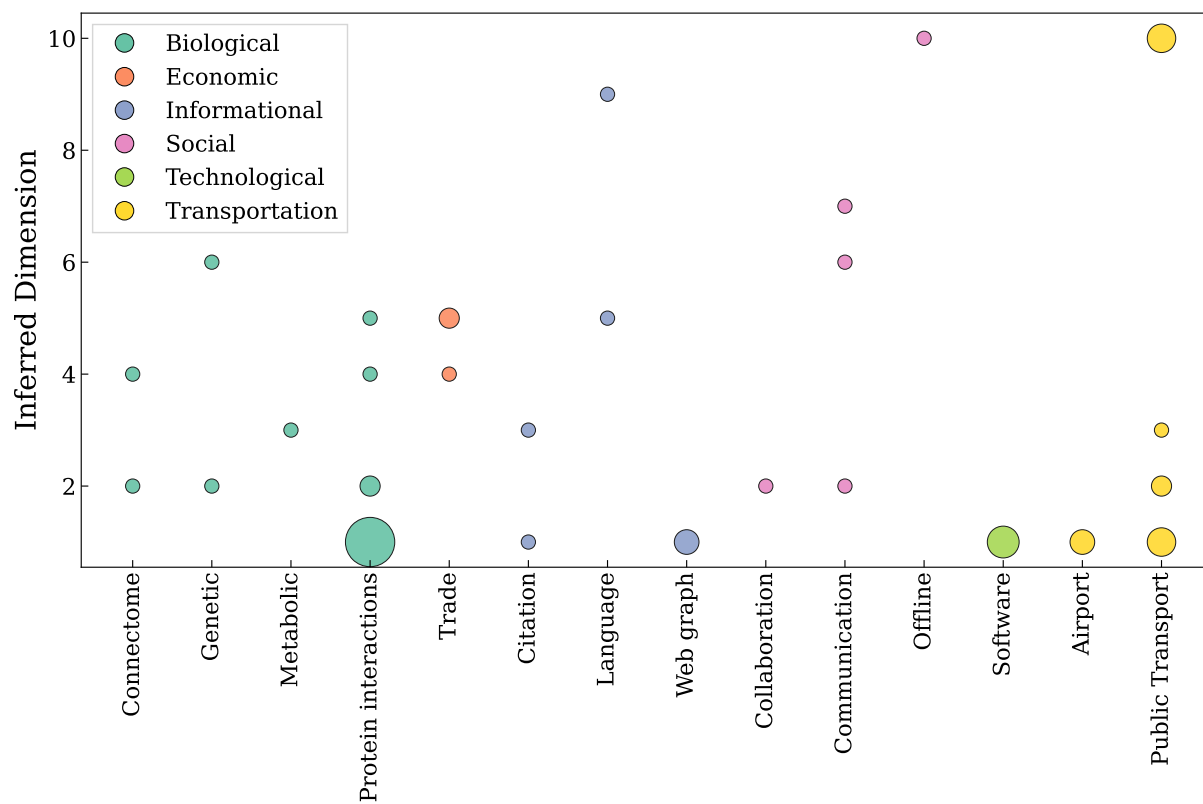

FIG. S7: Inferred dimension of real networks grouped by subdomain category.

TABLE S3: Properties of real networks, with network clustering, path and accuracy measures, and their dimensionality inferred with the DIMNN model. Part 1 of 2.

| Network                                          | Domain         | Subdomain            | $N$  | $\langle k \rangle$ | $\langle k \rangle^2 / \langle k \rangle^2$ | $k_{\min}$ | $k_{\max}$ |
|--------------------------------------------------|----------------|----------------------|------|---------------------|---------------------------------------------|------------|------------|
| Binary interactomes (various species; 2012)      | Biological     | Protein interactions | 974  | 4.72                | 3.52                                        | 1          | 55         |
| Uetz screen yeast interactome (2000)             | Biological     | Protein interactions | 263  | 2.14                | 1.86                                        | 1          | 17         |
| Reguly yeast interactome (2006)                  | Biological     | Protein interactions | 1213 | 4.21                | 2.11                                        | 1          | 40         |
| Ito core yeast interactome (2001)                | Biological     | Protein interactions | 426  | 2.45                | 3.44                                        | 1          | 56         |
| Yu yeast interactomes (2008)                     | Biological     | Protein interactions | 964  | 3.09                | 3.86                                        | 1          | 85         |
| C. elegans interactomes (2009)                   | Biological     | Protein interactions | 269  | 21.58               | 1.55                                        | 1          | 79         |
| Binary interactomes (musculus mouse; 2012)       | Biological     | Protein interactions | 537  | 3.83                | 2.99                                        | 1          | 59         |
| Binary interactomes (homo sapiens; 2012)         | Biological     | Protein interactions | 3155 | 3.58                | 3.31                                        | 1          | 131        |
| Binary interactomes (musculus mouse; 2012)       | Biological     | Protein interactions | 705  | 3.53                | 2.92                                        | 1          | 59         |
| C. elegans interactomes (2009)                   | Biological     | Protein interactions | 2214 | 3.20                | 4.50                                        | 1          | 99         |
| Binary interactomes (musculus mouse; 2012)       | Biological     | Protein interactions | 890  | 2.99                | 4.50                                        | 1          | 76         |
| C. elegans interactomes (scaffold, 2009)         | Biological     | Protein interactions | 345  | 2.32                | 2.67                                        | 1          | 28         |
| Yu yeast interactomes (2008)                     | Biological     | Protein interactions | 1647 | 3.06                | 3.82                                        | 1          | 89         |
| C. elegans interactomes (genetic, 2009)          | Biological     | Protein interactions | 683  | 4.52                | 2.39                                        | 1          | 56         |
| C. elegans interactomes (WI-2004, 2009)          | Biological     | Protein interactions | 1084 | 2.96                | 4.42                                        | 1          | 74         |
| C. elegans interactomes (WI-2007, 2009)          | Biological     | Protein interactions | 1108 | 2.71                | 4.42                                        | 1          | 84         |
| Human2-C                                         | Biological     | Connectome           | 496  | 32.41               | 1.17                                        | 1          | 80         |
| Human-M                                          | Biological     | Metabolic            | 1436 | 6.57                | 4.77                                        | 1          | 224        |
| Malaria var DBLa HVR networks                    | Biological     | Genetic              | 291  | 22.34               | 1.48                                        | 1          | 61         |
| Malaria var DBLa HVR networks                    | Biological     | Genetic              | 298  | 18.01               | 1.37                                        | 1          | 48         |
| Cargoships                                       | Economic       | Trade                | 821  | 10.58               | 3.12                                        | 1          | 173        |
| Atlas of Economic Complexity export network      | Economic       | Trade                | 774  | 4.59                | 2.70                                        | 1          | 43         |
| Atlas of Economic Complexity export network      | Economic       | Trade                | 866  | 5.85                | 2.81                                        | 1          | 48         |
| Garfield's citation networks (2001)              | Informational  | Citation             | 1024 | 9.60                | 3.95                                        | 1          | 232        |
| AMiner citation network (2009)                   | Informational  | Citation             | 1350 | 6.01                | 2.08                                        | 1          | 96         |
| Roget's Thesaurus (1879)                         | Informational  | Language             | 994  | 7.32                | 1.44                                        | 1          | 28         |
| Bible-CO                                         | Informational  | Language             | 1707 | 10.61               | 3.92                                        | 2          | 364        |
| WebKB graphs (1998)                              | Informational  | Web graph            | 269  | 3.60                | 4.36                                        | 1          | 74         |
| WebKB graphs (1998)                              | Informational  | Web graph            | 280  | 3.95                | 2.75                                        | 1          | 57         |
| WebKB graphs (1998)                              | Informational  | Web graph            | 343  | 4.04                | 5.43                                        | 1          | 129        |
| Friends-OFF                                      | Social         | Offline              | 2539 | 8.24                | 1.27                                        | 1          | 27         |
| Friends-ON                                       | Social         | Communication        | 2000 | 16.10               | 2.72                                        | 1          | 273        |
| EUEmail                                          | Social         | Communication        | 986  | 32.58               | 2.29                                        | 1          | 345        |
| Jazz-CA                                          | Social         | Collaboration        | 199  | 29.23               | 1.51                                        | 1          | 189        |
| Javax, Java, Jung, AppEngine dependencies (2010) | Technological  | Software             | 1031 | 8.55                | 3.29                                        | 1          | 208        |
| Software function-callgraphs (AbiWord, 2002)     | Technological  | Software             | 1035 | 3.32                | 3.27                                        | 1          | 89         |
| Software function-callgraphs (VTK, 2002)         | Technological  | Software             | 771  | 3.52                | 3.66                                        | 1          | 83         |
| Javax, Java, Jung, AppEngine dependencies (2010) | Technological  | Software             | 435  | 5.99                | 2.59                                        | 1          | 109        |
| Guava library dependencies (2012)                | Technological  | Software             | 457  | 4.05                | 3.85                                        | 1          | 62         |
| World subways (2009)                             | Transportation | Public Transport     | 266  | 2.32                | 1.17                                        | 1          | 7          |
| European airline network                         | Transportation | Airport              | 417  | 14.16               | 3.10                                        | 1          | 112        |
| FAA Preferred Routes (2010)                      | Transportation | Airport              | 1226 | 3.93                | 1.87                                        | 1          | 34         |
| US airport network (top 500; 2002)               | Transportation | Airport              | 500  | 11.92               | 4.51                                        | 1          | 145        |
| London Transport Network                         | Transportation | Public Transport     | 369  | 2.33                | 1.19                                        | 1          | 7          |
| India bus routes (2016)                          | Transportation | Public Transport     | 1103 | 3.90                | 1.68                                        | 1          | 54         |
| India bus routes (2016)                          | Transportation | Public Transport     | 1554 | 4.63                | 1.84                                        | 1          | 52         |
| India bus routes (2016)                          | Transportation | Public Transport     | 1087 | 5.43                | 3.41                                        | 1          | 183        |
| World subways (2009)                             | Transportation | Public Transport     | 217  | 2.41                | 1.22                                        | 1          | 9          |
| World subways (2009)                             | Transportation | Public Transport     | 392  | 2.23                | 1.11                                        | 1          | 6          |
| World subways (2009)                             | Transportation | Public Transport     | 299  | 2.38                | 1.22                                        | 1          | 8          |
| World subways (2009)                             | Transportation | Public Transport     | 209  | 2.30                | 1.16                                        | 1          | 7          |
| India bus routes (2016)                          | Transportation | Public Transport     | 1009 | 3.19                | 1.49                                        | 1          | 15         |
| World subways (2009)                             | Transportation | Public Transport     | 433  | 2.19                | 1.13                                        | 1          | 8          |

TABLE S4: Properties of real networks, with network clustering, path and accuracy measures, and their dimensionality inferred with the DIMNN model. Part 2 of 2.

| Network                                          | $C_t$  | $C_s$  | $C_p$  | $TP_t$   | $TP_s$   | $TP_p$ | Acc.  | $D$ |
|--------------------------------------------------|--------|--------|--------|----------|----------|--------|-------|-----|
| Binary interactomes (various species; 2012)      | 0.1220 | 0.1228 | 0.0031 | 77.7921  | 49.5511  | 1.5393 | 1.000 | 1   |
| Uetz screen yeast interactome (2000)             | 0.0262 | 0.0251 | 0.0020 | 1.7500   | 2.1659   | 0.2455 | 1.000 | 1   |
| Reguly yeast interactome (2006)                  | 0.6015 | 0.0761 | 0.0020 | 227.0699 | 107.9266 | 3.2453 | 0.970 | 2   |
| Ito core yeast interactome (2001)                | 0.1345 | 0.0875 | 0.0034 | 11.6167  | 15.8933  | 0.7123 | 1.000 | 1   |
| Yu yeast interactomes (2008)                     | 0.1217 | 0.1189 | 0.0015 | 39.2622  | 55.9388  | 1.0447 | 1.000 | 1   |
| C. elegans interactomes (2009)                   | 0.4635 | 0.1516 | 0.0021 | 149.4319 | 63.0049  | 0.7239 | 0.551 | 2   |
| Binary interactomes (musculus mouse; 2012)       | 0.1646 | 0.1508 | 0.0027 | 40.5982  | 50.2391  | 1.2342 | 1.000 | 1   |
| Binary interactomes (homo sapiens; 2012)         | 0.1933 | 0.1161 | 0.0013 | 301.0725 | 258.7704 | 3.5773 | 0.956 | 1   |
| Binary interactomes (musculus mouse; 2012)       | 0.1744 | 0.1392 | 0.0023 | 50.8065  | 55.3945  | 1.2488 | 0.993 | 1   |
| C. elegans interactomes (2009)                   | 0.0728 | 0.0519 | 0.0010 | 82.7588  | 70.5024  | 1.2652 | 1.000 | 1   |
| Binary interactomes (musculus mouse; 2012)       | 0.3684 | 0.0608 | 0.0015 | 82.2267  | 35.0576  | 0.9259 | 0.757 | 4   |
| C. elegans interactomes (scaffold, 2009)         | 0.0803 | 0.0360 | 0.0034 | 6.8333   | 3.9875   | 0.4651 | 1.000 | 1   |
| Yu yeast interactomes (2008)                     | 0.1236 | 0.0762 | 0.0013 | 76.3197  | 64.8148  | 1.7078 | 1.000 | 1   |
| C. elegans interactomes (genetic, 2009)          | 0.4244 | 0.0840 | 0.0019 | 153.5247 | 67.5384  | 1.5513 | 0.661 | 5   |
| C. elegans interactomes (WI-2004, 2009)          | 0.0843 | 0.0689 | 0.0011 | 38.5890  | 40.9450  | 0.6395 | 1.000 | 1   |
| C. elegans interactomes (WI-2007, 2009)          | 0.0727 | 0.0666 | 0.0015 | 30.0982  | 31.0904  | 0.7986 | 1.000 | 1   |
| Human2-C                                         | 0.5378 | 0.1061 | 0.0009 | 323.3771 | 114.7546 | 0.7963 | 0.825 | 2   |
| Human-M                                          | 0.5866 | 0.0770 | 0.0011 | 449.3374 | 177.3222 | 3.8313 | 0.987 | 3   |
| Malaria var DBLa HVR networks                    | 0.6054 | 0.1240 | 0.0018 | 179.7420 | 58.5849  | 1.0851 | 0.986 | 2   |
| Malaria var DBLa HVR networks                    | 0.4510 | 0.0710 | 0.0019 | 161.5944 | 31.7981  | 0.6912 | 0.870 | 6   |
| Cargoships                                       | 0.5482 | 0.0873 | 0.0014 | 326.5759 | 131.8263 | 2.1144 | 0.775 | 5   |
| Atlas of Economic Complexity export network      | 0.4882 | 0.0525 | 0.0022 | 109.7275 | 31.6048  | 1.5757 | 0.669 | 5   |
| Atlas of Economic Complexity export network      | 0.5089 | 0.0759 | 0.0019 | 165.7158 | 57.9047  | 1.7043 | 0.734 | 4   |
| Garfield's citation networks (2001)              | 0.3539 | 0.0842 | 0.0013 | 412.2120 | 162.5747 | 1.5339 | 1.000 | 1   |
| AMiner citation network (2009)                   | 0.3401 | 0.0841 | 0.0027 | 409.2855 | 152.9663 | 5.1329 | 0.789 | 3   |
| Roget's Thesaurus (1879)                         | 0.1964 | 0.0385 | 0.0018 | 307.8835 | 71.9862  | 2.8535 | 0.688 | 9   |
| Bible-CO                                         | 0.6259 | 0.0347 | 0.0005 | 596.0701 | 122.7898 | 1.5247 | 0.828 | 5   |
| WebKB graphs (1998)                              | 0.3710 | 0.0731 | 0.0046 | 45.2202  | 20.3393  | 1.4145 | 1.000 | 1   |
| WebKB graphs (1998)                              | 0.4226 | 0.1367 | 0.0034 | 39.4806  | 28.7375  | 1.2093 | 0.689 | 1   |
| WebKB graphs (1998)                              | 0.2513 | 0.1365 | 0.0040 | 57.6453  | 44.9548  | 1.7253 | 1.000 | 1   |
| Friends-OFF                                      | 0.1785 | 0.0282 | 0.0013 | 794.9442 | 144.4772 | 5.0352 | 0.712 | 10  |
| Friends-ON                                       | 0.5241 | 0.0543 | 0.0007 | 878.8888 | 227.5659 | 1.8765 | 0.996 | 7   |
| EUEmail                                          | 0.4735 | 0.1363 | 0.0009 | 572.1027 | 228.7467 | 1.1775 | 1.000 | 2   |
| Jazz-CA                                          | 0.7568 | 0.1201 | 0.0010 | 133.8771 | 69.7319  | 0.6359 | 0.994 | 2   |
| Javax, Java, Jung, AppEngine dependencies (2010) | 0.4270 | 0.1397 | 0.0021 | 498.0842 | 235.9069 | 4.8104 | 1.000 | 1   |
| Software function-callgraphs (AbiWord, 2002)     | 0.1398 | 0.0966 | 0.0037 | 78.2229  | 65.4463  | 2.6173 | 1.000 | 1   |
| Software function-callgraphs (VTK, 2002)         | 0.1555 | 0.0939 | 0.0034 | 67.1126  | 47.4782  | 1.7499 | 1.000 | 1   |
| Javax, Java, Jung, AppEngine dependencies (2010) | 0.4683 | 0.1547 | 0.0041 | 154.3303 | 103.4080 | 3.3866 | 0.996 | 1   |
| Guava library dependencies (2012)                | 0.6199 | 0.1396 | 0.0016 | 73.3721  | 55.9591  | 0.6418 | 0.976 | 1   |
| World subways (2009)                             | 0.0642 | 0.0284 | 0.0046 | 7.9000   | 4.9694   | 0.5619 | 0.389 | 10  |
| European airline network                         | 0.5508 | 0.1690 | 0.0018 | 165.0670 | 108.7857 | 1.2235 | 1.000 | 1   |
| FAA Preferred Routes (2010)                      | 0.1089 | 0.0527 | 0.0047 | 130.2926 | 70.0767  | 6.0710 | 0.930 | 1   |
| US airport network (top 500; 2002)               | 0.8137 | 0.0907 | 0.0004 | 117.4738 | 106.0472 | 0.7758 | 1.000 | 1   |
| London Transport Network                         | 0.0528 | 0.0315 | 0.0023 | 9.9000   | 7.4528   | 0.5900 | 1.000 | 1   |
| India bus routes (2016)                          | 0.2469 | 0.0568 | 0.0053 | 225.6782 | 83.1205  | 7.2559 | 0.524 | 2   |
| India bus routes (2016)                          | 0.2359 | 0.0735 | 0.0030 | 359.0307 | 158.5868 | 6.9280 | 0.581 | 2   |
| India bus routes (2016)                          | 0.3333 | 0.0691 | 0.0032 | 329.8021 | 135.2038 | 6.3026 | 0.758 | 3   |
| World subways (2009)                             | 0.0453 | 0.0150 | 0.0047 | 6.0000   | 2.3667   | 0.5911 | 0.575 | 10  |
| World subways (2009)                             | 0.0111 | 0.0031 | 0.0040 | 2.6667   | 1.1250   | 1.0887 | 0.964 | 10  |
| World subways (2009)                             | 0.0393 | 0.0265 | 0.0040 | 6.8333   | 5.0270   | 0.9486 | 0.448 | 10  |
| World subways (2009)                             | 0.0128 | 0.0179 | 0.0015 | 1.6667   | 2.3889   | 0.2475 | 1.000 | 1   |
| India bus routes (2016)                          | 0.1282 | 0.1001 | 0.0044 | 95.3556  | 77.7124  | 3.9028 | 0.845 | 1   |
| World subways (2009)                             | 0.0303 | 0.0015 | 0.0022 | 6.6667   | 0.2571   | 0.5071 | 1.000 | 1   |



#### 4. NETWORK GENERATION ALGORITHMS

---

**Algorithm 1**  $\mathbb{S}^D$  network generation algorithm

---

```

1: Input: Dimension  $D$ , number of nodes  $N$ , power-law exponent  $\gamma$ , average degree  $\langle \kappa \rangle$ , inverse temperature  $\beta$ 
2: Output: Graph  $G = (V, E)$  with nodes expressed in angular coordinates
3:  $V \leftarrow \{\}$ 
4:  $E \leftarrow \{\}$ 
5:  $\kappa_0 \leftarrow \langle k \rangle (\gamma - 2)(1 - N^{-1}) / [(\gamma - 1)(1 - N^{(2-\gamma)/(\gamma-1)})]$ 
6:  $\kappa_c \leftarrow \kappa_0 N^{1/(\gamma-1)}$ 
7: for  $i = 1$  to  $N$  do
8:    $\kappa_i \sim \rho(\kappa) = \kappa^{-\gamma} \kappa_0^{\gamma-1} (\gamma - 1) / (1 - (\kappa_c / \kappa_0)^{1-\gamma})$ 
9:    $\theta_i \sim \text{Uniform}([0, 2\pi))$ 
10:   $V \leftarrow V \cup \{\theta_i\}$ 
11: end for
12:  $\mu \leftarrow \beta \Gamma(D/2) \sin(D\pi/\beta) / (2\pi^{1+D/2} \langle k \rangle)$ 
13: for  $i = 1$  to  $N$  do
14:   for  $j = i + 1$  to  $N$  do
15:     $p_{ij} \leftarrow 1 / (1 + [R\Delta\theta_{ij} / (\mu\kappa_i\kappa_j)^{1/D}]^\beta)$ 
16:     $E \leftarrow E \cup \{(i, j)\}$  with probability  $p_{ij}$ 
17:   end for
18: end for

```

---



---

**Algorithm 2** Geometric randomization rewiring (D-GR)

---

```

1: Input: Graph  $G = (V, E)$ , dimension  $D$ , inverse temperature  $\beta$ 
2: Output: Graph  $G = (V, E)$  with rewired edges
3: for  $t = 1$  to  $10 \cdot |E|$  do
4:    $(i, j), (l, m) \sim \text{Uniform}(E)$  without replacement
5:    $\mathcal{L}_n / \mathcal{L}_c \leftarrow (\Delta\theta_{ij} \Delta\theta_{lm} / [\Delta\theta_{il} \Delta\theta_{jm}])^\beta$ 
6:   if  $\mathcal{L}_n / \mathcal{L}_c > 1$  then
7:      $E \leftarrow E \cup \{(i, m), (l, j)\} \setminus \{(i, j), (l, m)\}$ 
8:   else
9:      $E \leftarrow E \cup \{(i, m), (l, j)\} \setminus \{(i, j), (l, m)\}$  with probability  $\mathcal{L}_n / \mathcal{L}_c$ 
10:   end if
11:   if  $|\mathcal{L}_n / \mathcal{L}_c - 1| < 10^{-6}$  then
12:     break
13:   end if
14: end for

```

---

#### SUPPLEMENTARY REFERENCES

- [1] P. Almagro, M. Boguñá, and M. Á. Serrano, Nature Communications **13**, 6096 (2022)
- [2] A. Ghasemian, H. Hosseinmardi, and A. Clauset, IEEE Transactions on Knowledge and Data Engineering **32**, 1722 (2019)
